# Supplementary material for: WildlifeReID-10k: Wildlife re-identification dataset with 10k individual animals
Source: arXiv:2406.09211 source file (2025-04-15)
Supplement: Supplementary file 1 [file appendix.tex]

\newpage
\appendix
